# Supplementary material for: Three Qubit Randomized Benchmarking
Source: arXiv:1712.06550 ancillary file (2018-12-12)
Supplement: Supplementary file 1 [file threeq_supp.pdf]

# Supplementary Information for “Three-Qubit Randomized Benchmarking”

David C. McKay,<sup>\*</sup> Sarah Sheldon, John A. Smolin, Jerry M. Chow, and Jay M. Gambetta

*IBM T.J. Watson Research Center, Yorktown Heights, NY 10598, USA*

(Dated: December 12, 2018)

## DEVICE

Here we give additional details about the device used for the three-qubit RB experiment. An expanded schematic and optical image are shown in Fig. 1. As mentioned in the main text the device is comprised of three fixed-frequency superconducting transmon qubits (Q0,Q1,Q2) of frequencies (5.353,5.291,5.237) GHz coupled to a common 6.17GHz bus resonator. Each of the qubits has an anharmonicity of (-332,-322,-322) MHz. Each qubit has a separate readout resonator of frequency (6.789,6.738,6.686) GHz. The qubits are coupled to the to the bus with  $g/2\pi = (87,87,71)$  MHz.

In the main text we mention that there is a variability in  $T_1$  and  $T_2$  over the course of the experiment. In Fig. 2 we plot  $T_1$  and  $T_2$  versus time to show the extent of this variability. Understanding why these coherence parameters vary is an open question.

## GENERATING THE CLIFFORD GROUP

To generate the circuits for the 1- and 2- qubit Clifford gates, we use a simple circuit construction that optimizes the number of 2-qubit gates, CNOTs for example. Using this optimization an average of 1.5 CNOTs per Clifford gate are needed for the 2-qubit case. For the 3-qubit Cliffords we perform an exhaustive search over all possible short circuits for each 3-qubit Clifford to find the circuits with the smallest number of gates. To optimize the amount of memory needed to store these circuits we find circuits for the 1451520 element 3-qubit symplectic group and then use the fact that the 92897280 element 3-qubit Clifford group is the semidirect product of this symplectic group with the Pauli group to construct the full circuits on the fly. Given a list of circuits for all Clifford elements, it is straightforward to pick from the list at random and construct optimal circuits for sequences of Clifford gates. Between each Clifford a barrier is inserted in the corresponding OpenQASM code to prevent compiling away the complexity of the sequence. It is also necessary to compute the inverse of the sequence. This is done by computing the Clifford group element corresponding to the sequence which can be done efficiently using the techniques of Aaronson-Gottesman[1]. This element is then found in the complete list and its circuit run backwards is the required inverse circuit.

The Clifford group is first computed using a static set of primitive 1- and 2- qubit gates ( $r, r^\dagger, h, x, y, z$  and CNOT) which is then transformed into an experimental set of gate ( $\pi/2$  rotations and CNOT). Counting the number of gates in the sequence list gives the average number of 1-qubit gates (of finite duration) and 2-qubit CNOT gates per Clifford. However, to properly sequence a list of gates into a circuit, the circuit must obey barriers created by multi-qubit gates. Due to the finite duration of physical gates this will add idle time to the circuit which we count as additional 1-qubit gates. The number of gates per Clifford after enforcing the scheduling constraint is summarized in Table I.

## CALCULATING EPC AND EPG FROM RANDOMIZED BENCHMARKING

In randomized benchmarking we measure the decay of qubit polarization versus the number of Clifford gates in the sequence averaged over randomized sequences. This randomization over Cliffords means that the error map twirls to a depolarization channel. Therefore, the polarization decays as,

$$P_0 = A\alpha^M + B \quad (1)$$

where  $M$  is the number of Clifford gates and  $1 - \alpha$  is the depolarizing probability in the twirled map,

$$\Lambda[\rho] = \alpha\rho + \frac{(1 - \alpha)}{d}\mathcal{I} \quad (2)$$

$$= \sum_k A_k \rho A_k^\dagger \quad (3)$$

$$A_0 = \sqrt{\alpha + \frac{1 - \alpha}{d^2}}\mathcal{I} \quad (4)$$

$$A_i = \sqrt{\frac{\alpha}{d}}P_i \quad (5)$$

where  $d$  is the dimension and  $P_i$  are the non-identity Pauli operators. Each Clifford gate is composed of a set of primitive gates such as single-qubit  $\pi/2$  rotations and two-qubit controlled-not (CNOT) gates. Under the assumption that we can represent these gate errors as depolarizing maps then we can estimate the error per Clifford in higher dimensions by composition of the underlying depolarizing maps,

$$\Lambda_C[\rho] = \Lambda_{g1}[\rho] \circ \dots \Lambda_{gn}[\rho] \quad (6)$$

and then apply a twirl to  $\Lambda_C$ , which can be done using the procedure outlined in Ref. [2], to obtain  $\alpha_C$  for Eqn. 2. This procedure is not straightforward because some of the maps are depolarizing only on a subset of the full space (e.g. single qubit gates used for constructing a 2Q Clifford). A depolarizing map in a subspace can be constructed from Eqn. 3 by restricting the terms  $P_i$  to a specific subspace  $S$  (similarly  $d \rightarrow d_S$ ),

$$\Lambda[\rho] = \alpha\rho + \frac{1-\alpha}{d_S^2} \left( \rho + \sum_{P \in S} (P\rho P) \right) \quad (7)$$

where  $S$  is the Pauli subspace of the depolarization (e.g. for 1Q in a 2Q space this would be  $\{XI, YI, ZI\}$ ). Next, we need to compose all the maps. This is easiest done as a matrix multiplication of Pauli Transfer Matrices (Raulis,  $R_{ij} = \text{Tr}(P_i \Lambda[P_j])/d$ ). For depolarizing maps the Raulis are diagonal and given by,

$$R_{i,i} = \begin{cases} \alpha & \text{if } \exists P_j \in S \text{ s.t. } [P_i, P_j] \neq 0 \\ 1 & \text{else} \end{cases} \quad (8)$$

where the above condition means that  $R_{i,i} = \alpha$  if the elements of  $P_i$  in the subspace given by  $S$  are non-identity Paulis (e.g. if  $S$  is the subspace of qubit 1 Paulis in a 2Q space this would be all Pauli's *except*  $\{II, IX, IY, IZ\}$ ). Finally, we need to twirl the map which is given by the trace of the Rauli (except for the  $\{0,0\}$  element) divided by  $4^n - 1$ .

Here we will give concrete equations relating the  $\alpha$  parameters of the underlying gates to the  $\alpha$  for the 1Q, 2Q and 3Q Clifford gates. For 1Q Cliffords the relation is straightforward because the underlying gates are in the same dimensional space,

$$\alpha_{1Q,C} = \alpha_0^{N_1} \quad (9)$$

where  $N_1$  is the number of one-qubit gates required for each 1Q Clifford and  $\alpha_0$  is the depolarizing parameter of the primitive one-qubit gate. For two qubits,

$$\alpha_{2Q,C} = \frac{1}{5} \left( \alpha_0^{N_1/2} + \alpha_1^{N_1/2} + 3\alpha_0^{N_1/2} \alpha_1^{N_1/2} \right) \alpha_{01}^{N_2} \quad (10)$$

where  $\alpha_i$  is the  $\alpha$  for the one-qubit gates on qubit  $i$ ,  $N_1$  is the number of *total* one-qubit gates per 2Q Clifford,  $\alpha_{01}$  is the  $\alpha$  for the two-qubit primitive gate and  $N_2$  is the number of primitive two-qubit gates per 2Q Clifford. For three-qubits we need to consider two cases,

one in which there are three two-qubit gates and the other in which there are two. For three two-qubit gates (between Q0-Q1, Q0-Q2, Q1-Q2),

$$\alpha_{3Q,C} = \frac{1}{63} \left( 3\alpha_0^{N_1/3} \alpha_{01}^{N_2/3} \alpha_{02}^{N_2/3} + 3\alpha_1^{N_1/3} \alpha_{01}^{N_2/3} \alpha_{12}^{N_2/3} + 3\alpha_2^{N_1/3} \alpha_{02}^{N_2/3} \alpha_{12}^{N_2/3} + \dots \right. \\ \left. 9\alpha_{01}^{N_2/3} \alpha_{02}^{N_2/3} \alpha_{12}^{N_2/3} \left[ \alpha_0^{N_1/3} \alpha_1^{N_1/3} + \alpha_0^{N_1/3} \alpha_2^{N_1/3} + \dots \right. \right. \\ \left. \left. \alpha_1^{N_1/3} \alpha_2^{N_1/3} + 3\alpha_0^{N_1/3} \alpha_1^{N_1/3} \alpha_2^{N_1/3} \right] \right) \quad (11)$$

where  $\alpha_i$  is the  $\alpha$  for the one-qubit gates on qubit  $i$ ,  $N_1$  is the number of *total* one-qubit gates per 3Q Clifford,  $\alpha_{ij}$  is the  $\alpha$  for the two-qubit primitive gate between qubits  $i$  and  $j$  and  $N_2$  is the number of primitive two-qubit gates per 3Q Clifford. If there are only two two-qubit primitive gates then remove the appropriate gate from Eqn. 11 and change the exponent  $N_2/3$  to  $N_2/2$ .

We can also invert these expressions to get the primitive gate  $\alpha$  from the Clifford  $\alpha$  provided we make some approximation for the value of  $\alpha$  for the other primitive gates. For example, we can invert Eqn. 10 to get  $\alpha_{01}$  from the measured value of  $\alpha_{2Q,C}$  if we make an assumption for  $\alpha_0, \alpha_1$ . This is how we calculate the error per CNOT gate quoted in the main text where we assume the 1-qubit  $\alpha$  are measured from 1-qubit simultaneous RB. The inverted expression is,

$$\alpha_{01} = \left( \frac{5\alpha_{2Q,C}}{\alpha_0^{N_1/2} + \alpha_1^{N_1/2} + 3\alpha_0^{N_1/2} \alpha_1^{N_1/2}} \right)^{1/N_2}. \quad (12)$$

In the limit that the 1-qubit errors are negligible,

$$\alpha_{01} = \alpha_{2Q,C}^{1/N_2}. \quad (13)$$

## EXPANDED DATASET

Due to space constraints in the main text we were only able to provide the EPG (error per gate) from each of the RB experiments. In this section we give all the raw data parameters from each of the RB experiment in Table II. The raw data is given as the  $\alpha$  fit parameter to the RB curves. We also plot all the 3Q RB curves in Fig. 3.

## SIMULATION

We simulate the RB sequences by tracking the density matrix through the sequence starting in the ground state. For each time step of the simulation we first apply a unitary operator corresponding to the gates in the RB sequence, then we apply any non-ideal unitary operators (e.g., due to a  $ZZ$  interaction), then we apply a density matrix map for the  $T_1, T_2$  decoherence terms. In terms of the explicit maps,

$$\Lambda_{gate}[\rho] = U_g \cdot \rho \cdot U_g^\dagger \quad (14)$$

$$\Lambda_{ZZ}[\rho] = U_{ZZ} \cdot \rho \cdot U_{ZZ}^\dagger \quad (15)$$

$$\begin{aligned} \Lambda_{T_1, T_2}[\rho] = & \frac{1 - e^{-t/T_2}}{2} \mathbf{Z} \cdot \rho \cdot \mathbf{Z} + \frac{1 + e^{-t/T_2}}{2} \rho + \dots \\ & (1 - e^{-t/T_1})|0\rangle\langle 1| \cdot \rho \cdot |1\rangle\langle 0| - (1 - e^{-t/T_1})|1\rangle\langle 1| \cdot \rho \cdot |1\rangle\langle 1| \end{aligned} \quad (16)$$

where  $\mathbf{Z}$  is the Pauli-Z operator,  $1/T_2 = 1/T_\phi + 1/2T_1$  and  $\Lambda_{T_1, T_2}$  needs to be applied for each qubit and the operators are assumed to be tensor products with the identity in the other qubit spaces. Eqn. 16 can be derived from the Kraus operators,

$$\Lambda = \sum_{k=\{0,1,2\}} A_k \rho A_k^\dagger \quad (17)$$

$$A_0 = \begin{bmatrix} 1 & 0 \\ 0 & \sqrt{1 - \lambda - \gamma} \end{bmatrix} \quad (18)$$

$$A_1 = \begin{bmatrix} 0 & 0 \\ 0 & \sqrt{\lambda} \end{bmatrix} \quad (19)$$

$$A_2 = \begin{bmatrix} 0 & \sqrt{\gamma} \\ 0 & 0 \end{bmatrix} \quad (20)$$

$$\gamma = 1 - e^{-t/T_1} \quad (21)$$

$$\lambda = e^{-t/T_1} (1 - e^{-2t/T_\phi}) \quad (22)$$

In order to simulate the sequences in this way all gates must be divisible in time by a constant multiple to line up (in time) the gates on different channels. Therefore, we choose the single qubit gates to be 48 ns (they are 44 ns in the experiment) so that they are exactly  $1/5^{th}$  of a two-qubit gate. The minimum time step is 48 ns and we divide the unitary action of the CNOT gate into 5 steps,  $U_{CNOT} = (U_{CNOT/5})^5$  and so each time step is

$$\rho_{t+1} = \Lambda_{T_1, T_2, Q_0} \circ \Lambda_{T_1, T_2, Q_1} \circ \Lambda_{T_1, T_2, Q_2} \circ \Lambda_{ZZ, 01} \circ \Lambda_{ZZ, 02} \circ \Lambda_{ZZ, 12} \circ U_{g, Q_0} \circ U_{g, Q_1} \circ U_{g, Q_2}[\rho_t] \quad (23)$$

for all single gates, but for a two-qubit gates on, e.g. 0-1, the unitary gates will be  $U_{CNOT/5,Q0-Q1} \circ U_{g,Q2}[\rho_t]$ . The single qubit gate may be an identity if that qubit is idle while waiting for the operations on the other qubits to finish. We use the coherence numbers listed in the main text for the simulation. For calibration B we apply the  $ZZ$  unitary as  $U = e^{-i2\pi\zeta|11\rangle\langle 11|t}$  where  $\zeta$  are the  $ZZ$  numbers from the main text. For calibration A we add a  $Z$  shift equal to half the  $ZZ$ ,  $U = e^{-i2\pi\zeta(|11\rangle\langle 11| - |10\rangle\langle 10|/2 - |01\rangle\langle 01|)t}$ . The results are shown in Fig. 4 and show excellent agreement with the experimental data. This is strong evidence that the RB fidelity is dictated by standard coherence metrics and  $ZZ$  crosstalk only. This also supports the experimental result that differences in calibration procedures can lead to widely different three-qubit RB fidelities.

---

\* [dcmckay@us.ibm.com](mailto:dcmckay@us.ibm.com)

- [1] S. Aaronson and D. Gottesman, [Phys. Rev. A \*\*70\*\*, 052328 \(2004\)](#).
- [2] J. M. Gambetta, A. D. Córcoles, S. T. Merkel, B. R. Johnson, J. A. Smolin, J. M. Chow, C. A. Ryan, C. Rigetti, S. Poletto, T. A. Ohki, M. B. Ketchen, and M. Steffen, [Phys. Rev. Lett. \*\*109\*\*, 240504 \(2012\)](#).

## FIGURES

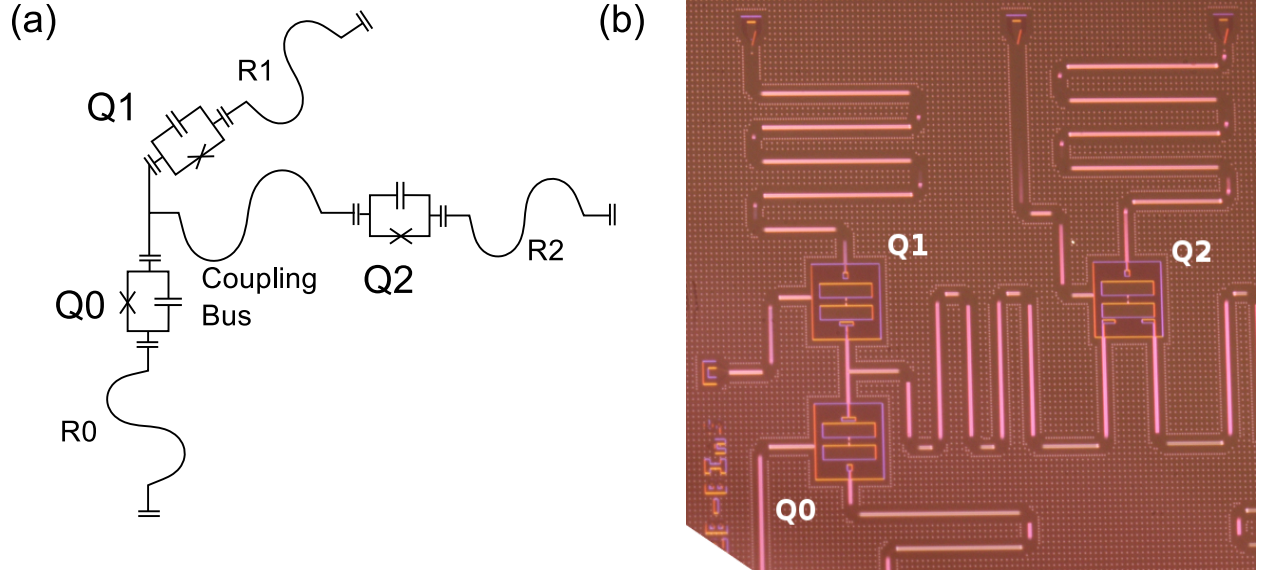

FIG. 1. (Color Online) (a) Schematic of the experimental setup, expanded from the figure in the main text to include the readout resonators. (b) Optical image of the device. Each qubit has an independent drive line; these were not used in the experiment as the qubits were driven through the readout resonators. The experiment was performed on 3 qubits out of a larger 5 qubit device, however, the extra 2 qubits were not operational. The device is niobium on silicon with Al-AlO<sub>2</sub>-Al junctions.

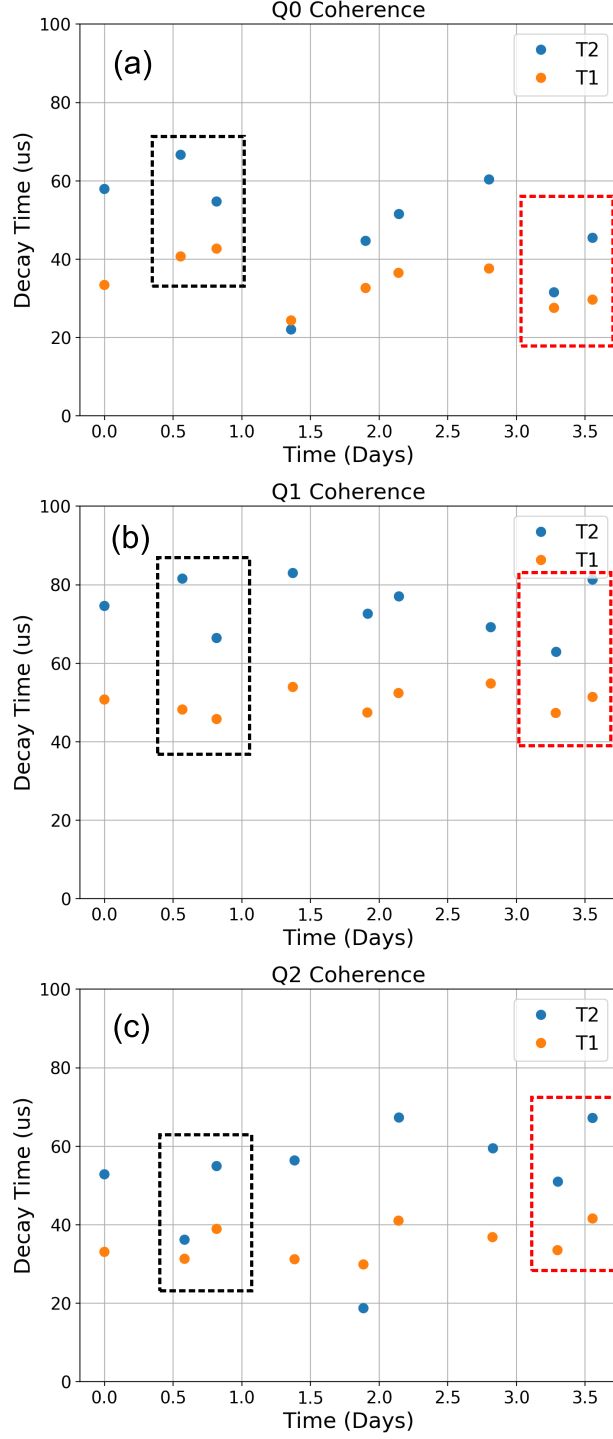

FIG. 2. (Color Online)  $T_1$  and  $T_2$  coherence data for (a) Q0, (b) Q1 and (c) Q2. The black box shows the coherence measurements before and after the RB taken for calibration B and the red box shows the measurements before and after the RB for calibration A.

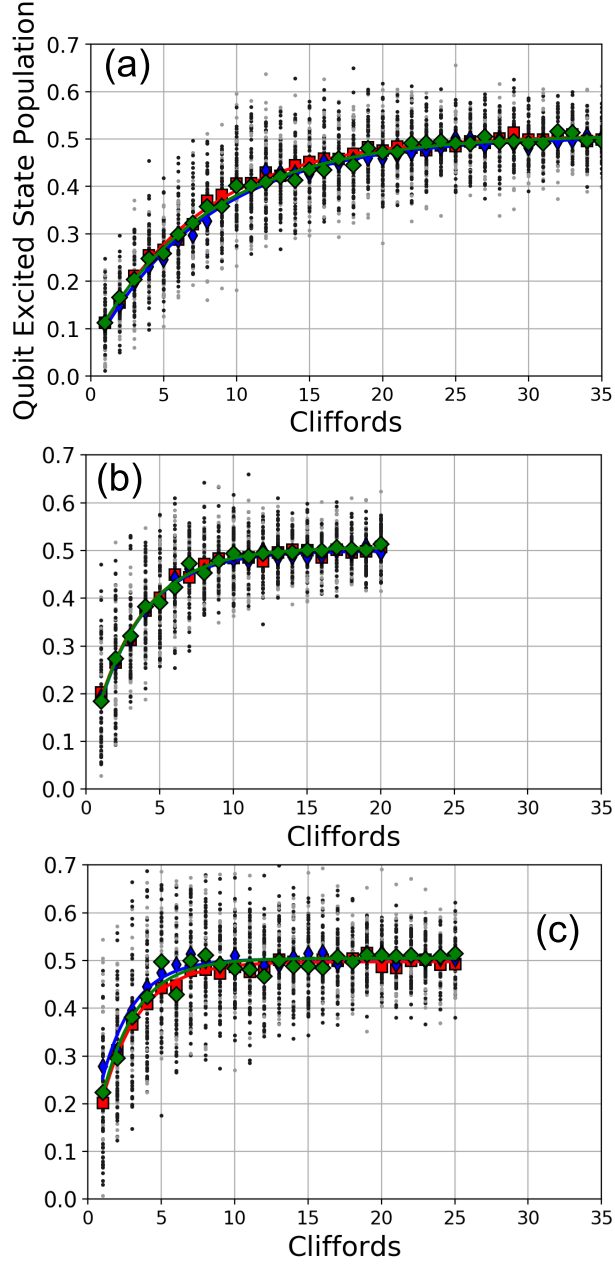

FIG. 3. (Color Online) Raw data from the different 3Q RB experiments as measured from Q0 (red), Q1 (blue) and Q2 (green). (a) Calibration A with all-to-all connectivity, (b) calibration A with limited connectivity and (c) calibration B with all-to-all connectivity.

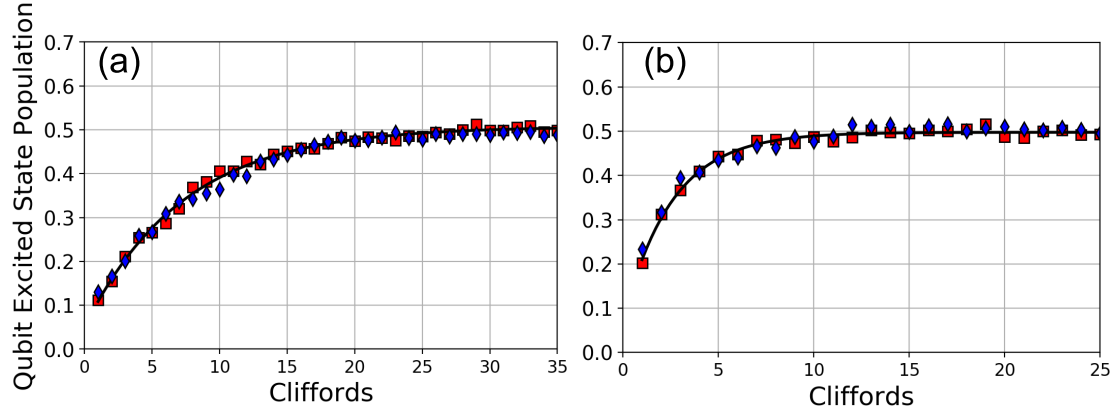

FIG. 4. (Color Online) Simulation (blue diamonds) compared to the experiment data measured by Q0 (red squares) for (a) calibration A and (b) calibration B. The black line is the fit to the experimental data.

## TABLES

| Clifford             | 1-Qubit Gates | 1-Qubit Gates (sequenced) | 2-Qubit Gates |
|----------------------|---------------|---------------------------|---------------|
| 1-Qubit              | 2.2083        | 2.2083                    | N/A           |
| 2-Qubit              | 12.2167       | 14.1                      | 1.5           |
| 3-Qubit (all-to-all) | 11.58         | 34.7                      | 3.51          |
| 3-Qubit (linear)     | 18.04         | 67.9                      | 7.716         |

TABLE I. The average number of 1- and 2-qubit gates per n-qubit Clifford for our gate construction. We give the number of 1-qubit gates in the list of gates and then after sequencing into a physical circuit.

|                                                                    | Cal. A                          | Cal. B                          |
|--------------------------------------------------------------------|---------------------------------|---------------------------------|
| Qubit Frequency Delta (kHz)                                        | [170,60,230]                    | [0,0,0]                         |
| $\alpha$ from $\{[0], [1], [2]\}$ RB                               | [0.9948(1),0.9962(1),0.9946(1)] | [0.9938(1),0.9964(1),0.9927(2)] |
| 1Q $\alpha$ from $\{[i], [j], [k]\}$ RB                            | [0.9938(1),0.9959(1),0.9941(1)] | [0.9926(1),0.9958(1),0.9932(1)] |
| 2Q $\alpha$ from $\{[i], [j]\}$ RB (control)                       | [0.952(1),0.950(1),0.928(3)]    | [0.963(1),0.927(3),0.955(2)]    |
| 2Q $\alpha$ from $\{[i], [j]\}$ RB (target)                        | [0.954(1),0.952(1),0.916(4)]    | [0.963(1),0.911(5),0.956(1)]    |
| 2Q $\alpha$ from $\{[i], [j], [k]\}$ RB (control)                  | [0.939(3),0.940(4),0.942(4)]    | [0.934(2),0.883(5),0.892(4)]    |
| 2Q $\alpha$ from $\{[i], [j], [k]\}$ RB (target)                   | [0.943(3),0.942(3),0.939(4)]    | [0.931(2),0.898(4),0.889(5)]    |
| 3Q $\alpha$ from $\{[0], [1], [2]\}$ RB (all-to-all)               | 0.872(5)/0.882(5)/0.883(4)      | 0.67(3)/0.64(4)/0.66(3)         |
| 3Q $\alpha$ from $\{[0], [1], [2]\}$ RB (omit CNOT <sub>12</sub> ) | 0.769(15)/0.761(15)/0.759(12)   | N/A                             |

TABLE II. Table of raw fit parameters for the data used in the main text. The qubit frequency is listed with respect to the calibration B frequencies [5.35298,5.29110,5.23733] GHz. The 3Q  $\alpha$  parameters are given as measured from the decay curve of  $Q0/Q1/Q2$ .
